# Supplementary material for: Kalai's $3^{d}$ conjecture for unconditional and locally anti-blocking polytopes
Source: arXiv:2308.02909 source file (2024-04-21)
Supplement: Supplementary file 1 [file appendix.tex]

\newpage
\appendix

\section{Code}

The following \texttt{SageMath} code was used to determine that $C(\Pi_3)$ has $97$ non-empty faces and $f$-vector $(12,36,36,12)$.

\vspace{1em}
\begin{verbatim}
    vectors = [
        ( 1, 1, 0, 0), ( 1,-1, 0, 0), (-1, 1, 0, 0), (-1,-1, 0, 0),
        ( 0, 1, 1, 0), ( 0, 1,-1, 0), ( 0,-1, 1, 0), ( 0,-1,-1, 0),
        ( 0, 0, 1, 1), ( 0, 0, 1,-1), ( 0, 0,-1, 1), ( 0, 0,-1,-1),
    ]
    poly = Polyhedron(vectors)
    
    # the f vector
    print(len(poly.faces(0)))
    print(len(poly.faces(1)))
    print(len(poly.faces(2)))
    print(len(poly.faces(3)))
    
    # the number of faces
    print(len(poly.face_lattice()) - 1)
    
\end{verbatim}

Note that $C(\Pi_3)$ is constructed using only the complete subgraphs of $\Pi_3$ of size~two (\ie\ the edges of $\Pi_3$).
The path has no larger complete subgraphs, and the complete subgraphs of cardinality one (\ie\ the vertices of $\Pi_3$) do not yield vertices of $C(\Pi_3)$ since each $e_i$ is included in the convex hull of $e_i+e_j$ and $e_i-e_j$ (where $j$ is so that $ij\in E(\Pi_3)$).
